# Supplementary material for: A Fourth-Generation High-Dimensional Neural Network Potential with Accurate Electrostatics Including Non-local Charge Transfer
Source: arXiv:2009.06484 ancillary file (2020-09-14)
Supplement: Supplementary file 1 [file Supplemental_Materials_of__Generalized_neural_network_potentials_with_accurate_electrostatic_interactions.pdf]

# Supplemental Materials for A Fourth-Generation High-Dimensional Neural Network Potential with Accurate Electrostatics Including Non-local Charge Transfer

Tsz Wai Ko, Jonas A Finkler, Stefan Goedecker, Jörg Behler

September 14, 2020

## Contents

**1 Methodical details** **2**
1.1 Overview . . . 2
1.2 Charge equilibration . . . 2
1.3 Derivatives used for the calculation of the forces and for the neural network training . . . 3
1.3.1 Calculation of $\frac{dQ_i}{dr_\alpha}$ . . . 4
1.3.2 Calculation of $\frac{dQ_i}{d\chi_i}$ and $\frac{dQ_i}{dJ_i}$ . . . 4
1.3.3 An efficient method for the force computation . . . 4
1.4 Charge equilibration for periodic systems . . . 5
1.5 Calculation of $\frac{dA_{ij}}{dr_\alpha}$ . . . 6
1.6 Short-range part . . . 7

**2 Additional information for test systems** **8**
2.1 $C_{10}H_2/C_{10}H_3^+$ . . . 8
2.2 $Ag_3^{+/-}$ clusters . . . 11
2.3 $Na_{8/9}Cl_8^+$ clusters . . . 13
2.4 $Au_2{-}MgO$ . . . 16

**3 DFT-optimized geometries** **21**
3.1 $C_{10}H_2/C_{10}H_3^+$ . . . 21

# 1 Methodical details

## 1.1 Overview

Here, we provide the technical details of the 4G-HDNNP method. The total energy consists of two parts, the short-range energy and long-range electrostatic energy,

$$E_{\text{total}} = E_{\text{elec}} + E_{\text{short}} \quad . \tag{1}$$

The electrostatic energy is calculated from the atomic charges, which are obtained from a charge equilibration scheme (Qeq) based on environment-dependent electronegativities that are predicted by atomic neural networks. The short-range energy is a sum of atomic energies computed by atomic neural networks, which compared to 2D-HDNNPs have an additional input node providing the atomic charge. With this additional information the short-range atomic neural networks are able to accurately predict energetic changes due to modifications in the local electronic structure resulting from long-range charge transfer. Atomic forces are calculated by taking the negative analytic derivatives of the total energy in Eq. 1 with respect to the atomic positions.

## 1.2 Charge equilibration

The charge equilibration method [1] is based on the idea that the electrons in a system are distributed in a way that minimizes the total energy. This energy does not only include the electrostatic Coulomb terms but also a term that describes the local energy caused by some amount of charge on an atom. This local energy is usually described using a Taylor series up to second order. The expansion factor for the linear term is called the electronegativity ($\chi_i$), while the second order factor is called the atomic hardness ($J_i$). The charge on each atom is Gaussian distributed with width $\sigma_i$. This results in the energy expression for the charge equilibration scheme

$$E_{\text{Qeq}} = E_{\text{elec}} + \sum_{i=1}^{N_{\text{at}}} \chi_i Q_i + \frac{1}{2} J_i Q_i^2 \quad . \tag{2}$$

$N_{\text{at}}$ is the number of atoms in the system. $E_{\text{elec}}$ is the electrostatic energy resulting from the Gaussian charge distributions,

$$E_{\text{elec}} = \sum_{\text{i<j}}^{N_{\text{at}}} \frac{\operatorname{erf}\left(\frac{r_{ij}}{\sqrt{2}\gamma_{ij}}\right)}{r_{ij}} Q_i Q_i + \sum_{i=1}^{N_{\text{at}}} \frac{Q_i^2}{2\sigma_i\sqrt{\pi}} \tag{3}$$

and

$$\gamma_{ij} = \sqrt{\sigma_i^2 + \sigma_j^2} \quad . \tag{4}$$

As only linear and quadratic terms in $Q_i$ appear in $E_{\text{elec}}$ and $E_{\text{Qeq}}$, they can be expressed using matrix notation

$$[\mathbf{E}]_{ij} = \begin{cases} \frac{1}{\sigma_i\sqrt{\pi}}, & \text{if } i = j \\ \frac{\operatorname{erf}\left(\frac{r_{ij}}{\sqrt{2}\gamma_{ij}}\right)}{r_{ij}}, & \text{otherwise} \end{cases} \tag{5}$$

$$E_{\text{elec}} = \frac{1}{2}\mathbf{Q}^\top \mathbf{E} \mathbf{Q} \tag{6}$$

and

$$E_{\text{Qeq}} = \frac{1}{2}\mathbf{Q}^\top \mathbf{A} \mathbf{Q} + \mathbf{Q}^\top \boldsymbol{\chi} \quad , \tag{7}$$

with $\mathbf{Q}$ being a column vector containing the atomic charges $Q_i$, $\boldsymbol{\chi}$ being a column vector of the electronegativities and $\mathbf{A}$ being the matrix

$$[\mathbf{A}]_{ij} = \begin{cases} J_i + \frac{1}{\sigma_i\sqrt{\pi}}, & \text{if } i = j \\ \frac{\mathrm{erf}\left(\frac{r_{ij}}{\sqrt{2}\gamma_{ij}}\right)}{r_{ij}}, & \text{otherwise} \end{cases} \quad . \tag{8}$$

It has to be noted that because the total energy of a continuous charge distribution is always positive, the matrix $\mathbf{A}$ is positive definite, if the $J_i > 0$.

The $Q_i$ are now chosen, so that they minimize the energy $E_{\mathrm{Qeq}}$ under the additional constraint of total charge conservation

$$\sum_{i=1}^{N_{\mathrm{at}}} Q_i = Q_{\mathrm{tot}} \quad . \tag{9}$$

To solve this minimization problem, we set the derivatives with respect to the charges to zero,

$$\frac{dE_{\mathrm{Qeq}}}{dQ_i} = 0 \quad . \tag{10}$$

Including the constraint of total charge conservation using a Lagrange multiplier $\lambda$ we end up with the system of linear equations

$$\left(\begin{array}{ccc|c} & & & 1 \\ & \mathbf{A} & & \vdots \\ & & & 1 \\ \hline 1 & \dots & 1 & 0 \end{array}\right) \left(\begin{array}{c} Q_1 \\ \vdots \\ Q_{N_{\mathrm{at}}} \\ \hline \lambda \end{array}\right) = \left(\begin{array}{c} -\chi_1 \\ \vdots \\ -\chi_{N_{\mathrm{at}}} \\ \hline Q_{\mathrm{tot}} \end{array}\right) \quad , \tag{11}$$

which we can rewrite for simplicity as

$$\mathbf{A}'\mathbf{Q}' = \mathbf{b} \quad , \tag{12}$$

where $\mathbf{A}'$ and $\mathbf{Q}'$ represent the $(N_{\mathrm{at}} + 1 \times N_{\mathrm{at}} + 1)$ matrix and column vector in the left hand side respectively, while $\mathbf{b}$ is the column vector on the right hand side. The electronegativities $\chi_i$ are predicted by neural networks, for each atom individually, depending on the local chemical environments. The hardness values of $J_i$ are constant for a given element, and they are also optimized during the training of the neural networks.

## 1.3 Derivatives used for the calculation of the forces and for the neural network training

In this section we provide further details about some of the derivatives which are required for the calculation of the atomic forces as well as for the gradient-based optimization of the neural network parameters. The atomic force component $F_{r_\alpha}$ is given as the negative derivative of the energy with respect to the atomic coordinate $r_\alpha$,

$$F_{r_\alpha} = -\frac{dE_{\mathrm{total}}(\mathbf{R}, \mathbf{Q}(\mathbf{R}))}{dr_\alpha} = \frac{\partial E_{\mathrm{total}}}{\partial r_\alpha} - \sum_i \frac{\partial E_{\mathrm{total}}}{\partial Q_i}\frac{\partial Q_i}{\partial r_\alpha} \quad . \tag{13}$$

In this equation the partial derivatives of the atomic charges with respect to the atomic positions appear. As we will show in section 1.3.3, the calculation of these terms can be avoided for the determination of the forces. During the training phase, however, these derivatives as well as the derivatives of the charges w.r.t. the electronegativity and hardness are needed.

### 1.3.1 Calculation of $\frac{dQ_i}{dr_\alpha}$

To calculate the $\frac{\partial Q_i}{\partial r_\alpha}$ we take the derivative with respect to the spatial coordinate $r_\alpha$ of the Qeq Eq. 12. Reordering the terms yields

$$\mathbf{A}\frac{\partial \mathbf{Q}}{\partial r_\alpha} = \frac{-\partial \boldsymbol{\chi}}{\partial r_\alpha} - \frac{\partial \mathbf{A}}{\partial r_\alpha}\mathbf{Q} \tag{14}$$

as well as a Lagrange multiplier that ensures $\sum_i \frac{\partial Q_i}{\partial r_\alpha} = 0$. To obtain all the $3N_{\mathrm{at}}$ required derivatives we will have to solve 3 $N_{\mathrm{at}}$ linear equation systems of size $N_{\mathrm{at}}+1$. However, this can be avoided as explained in section 1.3.3, which allows the calculation of the total force by only solving one linear equation system.

### 1.3.2 Calculation of $\frac{dQ_i}{d\chi_i}$ and $\frac{dQ_i}{dJ_i}$

With an similar procedure we can calculate the equation systems for the derivatives w.r.t. the electronegativity and hardness

$$\mathbf{A}\frac{d\mathbf{Q}}{d\chi_i} = -\boldsymbol{\delta}_i \tag{15}$$

and

$$\mathbf{A}\frac{d\mathbf{Q}}{dJ_i} = -\mathbf{Q} \quad . \tag{16}$$

$\boldsymbol{\delta}_i$ is a vector filled with zeros except entry $i$, which is one. As before, a Lagrange multiplier will be necessary, to ensure that the sum of the derivatives adds up to zero.

### 1.3.3 An efficient method for the force computation

In the last section we showed how the forces can be calculated using the partial derivatives of the charges w.r.t. the atomic coordinates. This calculation is computationally expensive, since 3 $N_{\mathrm{at}}$ linear equation systems need to be solved. This can be avoided by exploiting a method [2] that allows the calculation of the forces by solving only one linear equation system instead.

The total energy of the 4G-HDNNP is a function of the atomic coordinates ($\mathbf{R}$) and the charges ($\mathbf{Q}$), which also depend on the atomic coordinates,

$$E_{\mathrm{total}} = E_{\mathrm{total}}(\mathbf{R}, \mathbf{Q}(\mathbf{R})) \quad . \tag{17}$$

We now define an auxiliary function $L$ with

$$L = E_{\mathrm{total}} + \sum_{i=1}^{N_{\mathrm{at}}+1} \lambda_i \left( \sum_{j=1}^{N_{\mathrm{at}}+1} A'_{ij} Q'_j - b_i \right) \quad . \tag{18}$$

Here $\sum_{j=1}^{N_{\mathrm{at}}+1} A'_{ij} Q'_j - b_i$ are the differences of the left hand side minus the right hand sides of Eq. 12, which were solved to determine the charges $Q_i$. These terms are therefore always zero, making $L$ equal to $E_{\mathrm{total}}$. We now choose $\lambda$ such that the partial derivatives $\frac{\partial L}{\partial Q'_i}$ are zero,

$$\frac{\partial L}{\partial Q'_i} = \frac{\partial E_{\mathrm{total}}}{\partial Q'_i} + \sum_{j=1}^{N_{\mathrm{at}}+1} A'_{ij}\lambda_j = 0 \quad . \tag{19}$$

For this we solve the linear equation system

$$\sum_{j=1}^{N_{\mathrm{at}}+1} A'_{ij}\lambda_j = \frac{-\partial E_{\mathrm{total}}}{\partial Q'_i} \quad . \tag{20}$$

Note that $\mathbf{A}'$ is a symmetric matrix. We now turn to the derivative $\frac{dL}{dr_\alpha}$, which is equal to $\frac{dE_{\mathrm{total}}}{dr_\alpha}$.

$$\frac{dE_{\mathrm{total}}}{dr_\alpha} = \frac{dL}{dr_\alpha} = \frac{\partial E_{\mathrm{total}}}{\partial r_\alpha} + \sum_{i=1}^{N_{\mathrm{at}}+1} \frac{\partial E_{\mathrm{total}}}{\partial Q'_i}\frac{\partial Q'_i}{\partial r_\alpha} + \sum_{i=1}^{N_{\mathrm{at}}+1} \lambda_i \left( \sum_{j=1}^{N_{\mathrm{at}}+1} \frac{\partial A'_{ij}}{\partial r_\alpha} Q'_j + \sum_{j=1}^{N_{\mathrm{at}}+1} A'_{ij} \frac{\partial Q'_j}{\partial r_\alpha} - \frac{\partial b_i}{\partial r_\alpha} \right) \tag{21}$$

Rearranging the equation yields

$$\frac{dE_{\mathrm{total}}}{dr_\alpha} = \frac{dL}{dr_\alpha} = \frac{\partial E_{\mathrm{total}}}{\partial r_\alpha} + \sum_{i=1}^{N_{\mathrm{at}}+1} \left( \frac{\partial E_{\mathrm{total}}}{\partial Q'_i} + \sum_{j=1}^{N_{\mathrm{at}}+1} A'_{ij}\lambda_j \right) \frac{\partial Q'_i}{\partial r_\alpha} + \sum_{i=1}^{N_{\mathrm{at}}+1} \lambda_i \left( \sum_{j=1}^{N_{\mathrm{at}}+1} \frac{\partial A'_{ij}}{\partial r_\alpha} Q'_j - \frac{\partial b_i}{\partial r_\alpha} \right) \quad . \tag{22}$$

The term $\frac{\partial E_{\mathrm{total}}}{\partial Q'_i} + \sum_j A'_{ij}\lambda_j$ is zero by definition of $\lambda$ and can therefore be omitted, which leads to the expression

$$\frac{dE_{\mathrm{total}}}{dr_\alpha} = \frac{\partial E_{\mathrm{total}}}{\partial r_\alpha} + \sum_{i=1}^{N_{\mathrm{at}}+1} \lambda_i \left( \sum_{j=1}^{N_{\mathrm{at}}+1} \frac{\partial A'_{ij}}{\partial r_\alpha} Q'_j - \frac{\partial b_i}{\partial r_\alpha} \right) \quad . \tag{23}$$

## 1.4 Charge equilibration for periodic systems

The Qeq equations for periodic boundary conditions are essentially identical to the corresponding equations for free boundary conditions, and the main difference is the calculation of the matrix $\mathbf{A}$. Because of the periodic boundary conditions we have to resort to an Ewald summation [3] to calculate the electrostatic interaction energy.

The basic idea of Ewald summation is, that by placing Gaussian charges of the opposite sign on each of the point charges, the remaining electrostatic interaction becomes short-ranged. This short-ranged energy can then be calculated in real space ($E_{\mathrm{real}}$). We then subtract the interaction energy of the auxiliary Gaussian charges again to obtain the desired total energy of the point charges. This interaction energy of the Gaussians can be efficiently calculated in reciprocal space, resulting in the energies $E_{\mathrm{recip}}$ and $E_{\mathrm{self}}$. The electrostatic energy of $N_{\mathrm{at}}$ point charges can be hence calculated as

$$E_{\mathrm{elec}} = E_{\mathrm{real}} + E_{\mathrm{recip}} + E_{\mathrm{self}} \quad . \tag{24}$$

The real space part is given by

$$E^{\mathrm{pc}}_{\mathrm{real}} = \frac{1}{2} \sum_{i=1}^{N_{\mathrm{at}}} \sum_{j \neq i}^{N_{\mathrm{neig}}} Q_i Q_j \frac{\mathrm{erfc}\left(\frac{r_{ij}}{\sqrt{2}\eta}\right)}{r_{ij}} \tag{25}$$

Here, $N_{\mathrm{neig}}$ indicates, that the sum goes over all neighbouring atoms withing the real space cutoff radius $r_{\mathrm{cut}}$. $r_{ij}$ is the distance between atoms $i$ and $j$. The reciprocal space part is

$$E^{\mathrm{pc}}_{\mathrm{recip}} = \frac{2\pi}{V} \sum_{\mathbf{k}\neq 0} \frac{\exp\left(\frac{-\eta^2|\mathbf{k}|^2}{2}\right)}{|\mathbf{k}|^2} |S(\mathbf{k})|^2 \tag{26}$$

with

$$S(\mathbf{k}) = \sum_{i=1}^{N_{\text{at}}} Q_i \exp(i\mathbf{k} \cdot \mathbf{r}_i) \tag{27}$$

$V$ being the volume of the unit cell and the sum going over all reciprocal lattice points inside reciprocal space cutoff radius $r_{\text{cut}}^{\text{recip}}$. Finally, the self-interaction correction is

$$E_{\text{self}}^{\text{pc}} = -\sum_{i=1}^{N_{\text{at}}} \frac{Q_i^2}{\sqrt{2\pi}\eta} \tag{28}$$

In these equations $\eta$ is the standard deviation of the Gaussian charges, which are placed on the point charges to remove the long-range interactions.

Since we use Gaussian charge distributions for the charge equilibration process, the following terms have to be added that account for the different interaction in the short-range part as well as for the self interaction of the Gaussian charges [4, 5, 6].

$$E_{\text{elec}}^{\text{Gauss}} = E_{\text{elec}}^{\text{pc}} - \frac{1}{2} \sum_{i=1}^{N_{\text{at}}} \sum_{j \neq i}^{N_{\text{neig}}} Q_i Q_j \frac{\operatorname{erfc}\left(\frac{r_{ij}}{\sqrt{2}\gamma}\right)}{r_{ij}} + \sum_{i=1}^{N_{\text{at}}} \frac{Q_i^2}{2\sqrt{\pi}\sigma_i} \tag{29}$$

Here $E_{\text{elec}}^{\text{pc}}$ is the electrostatic energy of the point charges as given above.

The important observation is that the total energy expression of the Ewald summation contains only terms of the form $\frac{1}{2}e_{ij}Q_iQ_j$. By calculating the individual coefficients $e_{ij}$ we can therefore construct the matrix $\mathbf{E}$, so that

$$E_{\text{elec}} = \frac{1}{2}\mathbf{Q}^{\top}\mathbf{E}\mathbf{Q} \quad . \tag{30}$$

Including the terms for the hardness and adding the electronegativity results in a formalism equivalent to that of the Qeq method for free boundary condition.

## 1.5 Calculation of $\frac{dA_{ij}}{dr_\alpha}$

The differentiation of the above equation allows us to calculate the derivatives $\frac{dA_{ij}}{dr_\alpha}$. Explicit calculation of these derivatives however can be computationally expensive, as they are quite numerous ($3N_{\text{at}}^3$). Most of these coefficients however are zero, and the matrix is very sparse. As only the product $\sum_{j=1} \frac{dA_{ij}}{dr_\alpha} Q_j$ is ever needed in our computations, explicit calculation can be avoided and only the non zero terms have to be considered.

As $\sum_{j=1} \frac{dA_{ij}}{dr_\alpha} Q_j$ has to be calculated anyways for the efficient compuations of the forces, we can also use it to calculate the electrostatic forces.

$$\frac{\partial E_{\text{elec}}}{\partial r_\alpha} = \frac{1}{2} \sum_i Q_i \left( \sum_j \frac{dA_{ij}}{dr_\alpha} Q_j \right) \tag{31}$$

Calculation of the electrostatic energies and forces boils down to the following.

1. Calculate symmetry functions
2. Calculate environment depend electronegativities using a first set of neural networks
3. Construct the matrix $\mathbf{A}$

4. Calculate partial charges $Q_i$ by solving the system of $N_{\mathrm{at}}$+1 linear equations (Eq. 11)
5. Feed the atomic charges into the atomic NNs to calculate the short range energy and forces
6. Use the efficient method (section 1.3.3) to calculate the total force by solving one more $N_{\mathrm{at}} + 1$ dimensional linear equation system.

The only difference for the periodic case is in the step 3 and 6, where Ewald summation has to be used.

## 1.6 Short-range part

In the short range neural network, we also include the atomic charge via an additional input neuron, such that the atomic energy contribution also depends on global charge distributions. The expression of atomic energies is very similar to the 2G-HDNNP and it can be expressed as a function of symmetry functions and atomic charges. The atomic forces can be calculated by taking the derivatives of the energy with respect to the atomic positions

$$F_\alpha = -\sum_{i=1}^{N_{\mathrm{at}}} \frac{dE_i}{dr_\alpha} = -(\sum_{j=1}^{N_{\mathrm{neig},i}} \sum_{k=1}^{N_{\mathrm{SF},j}} \frac{\partial E_j}{\partial G_{j,k}} \cdot \frac{\partial G_{j,k}}{\partial r_\alpha} + \sum_{j=1}^{N_{\mathrm{at}}} \sum_{k=1}^{N_{\mathrm{at}}} \frac{\partial E_j}{\partial Q_k} \cdot \frac{\partial Q_k}{\partial r_\alpha}) \tag{32}$$

where $F_\alpha$ and $G_{j,k}$ represent the force component $\alpha$ and the $k^{\mathrm{th}}$ symmetry function of atom $j$ respectively. In addition, $N_{\mathrm{SF},i}$, $N_{\mathrm{neig},i}$ equal to number of symmetry functions and neighbors of atom $i$ and $N_{\mathrm{at}}$ the total number of atom. Note that $N_{\mathrm{neig},i}$ includes the atom $i$ itself. If the method described in section 1.3.3 is used, the last term, which includes the partial derivatives of the atomic charges w.r.t. the atomic coordinates, can be avoided.

# 2 Additional information for test systems

## 2.1 $C_{10}H_2/C_{10}H_3^+$

Table 1: Root mean square errors (RMSE) of charges (me), energies (meV/atom) and forces (meV/Å) for the three different HDNNP generations for the $C_{10}H_2/C_{10}H_3^+$ data set with 9035 and 984 structures for training and testing points respectively.

| | | charges | energy | forces |
|---|---|---|---|---|
| 2G | train | — | 1.583 | 130.7 |
| | test | — | 1.619 | 129.5 |
| 3G (unscaled) | train | 27.36 | 3.192 | 652.5 |
| | test | 27.35 | 3.197 | 658.3 |
| 3G (scaled) | train | 19.98 | 2.017 | 229.9 |
| | test | 20.08 | 2.045 | 231.0 |
| 4G | train | 5.783 | 1.148 | 77.65 |
| | test | 6.577 | 1.194 | 78.00 |

Table 2: Symmetry functions for $C_{10}H_2/C_{10}H_3^+$

| no. | type | atom i | atom j | atom k | $\eta$(1/Bohr$^2$) | $\lambda$ | $\zeta$ | R$_c$(Bohr) | R$_s$(Bohr) |
|---|---|---|---|---|---|---|---|---|---|
| 1 | 2 | H | H | | 0.0 | | | 8.0 | 0.0 |
| 2 | 2 | H | H | | 0.006 | | | 8.0 | 0.0 |
| 3 | 2 | H | H | | 0.011 | | | 8.0 | 0.0 |
| 4 | 2 | H | H | | 0.018 | | | 8.0 | 0.0 |
| 5 | 2 | H | H | | 0.026 | | | 8.0 | 0.0 |
| 6 | 2 | H | H | | 0.035 | | | 8.0 | 0.0 |
| 7 | 2 | C | H | | 0.0 | | | 8.0 | 0.0 |
| 8 | 2 | C | H | | 0.013 | | | 8.0 | 0.0 |
| 9 | 2 | C | H | | 0.029 | | | 8.0 | 0.0 |
| 10 | 2 | C | H | | 0.054 | | | 8.0 | 0.0 |
| 11 | 2 | C | H | | 0.093 | | | 8.0 | 0.0 |
| 12 | 2 | C | H | | 0.161 | | | 8.0 | 0.0 |
| 13 | 2 | H | C | | 0.0 | | | 8.0 | 0.0 |
| 14 | 2 | H | C | | 0.013 | | | 8.0 | 0.0 |
| 15 | 2 | H | C | | 0.029 | | | 8.0 | 0.0 |
| 16 | 2 | H | C | | 0.054 | | | 8.0 | 0.0 |
| 17 | 2 | H | C | | 0.093 | | | 8.0 | 0.0 |
| 18 | 2 | H | C | | 0.161 | | | 8.0 | 0.0 |
| 19 | 2 | C | C | | 0.0 | | | 8.0 | 0.0 |
| 20 | 2 | C | C | | 0.01 | | | 8.0 | 0.0 |
| 21 | 2 | C | C | | 0.023 | | | 8.0 | 0.0 |
| 22 | 2 | C | C | | 0.041 | | | 8.0 | 0.0 |

| no. | type | atom i | atom j | atom k | $\eta$(1/Bohr$^2$) | $\lambda$ | $\zeta$ | R$_c$(Bohr) | R$_s$(Bohr) |
|---|---|---|---|---|---|---|---|---|---|
| 23 | 2 | C | C | | 0.065 | | | 8.0 | 0.0 |
| 24 | 2 | C | C | | 0.103 | | | 8.0 | 0.0 |
| 25 | 3 | C | C | C | 0.0 | 1.0 | 1.0 | 8.0 | |
| 26 | 3 | C | C | C | 0.0 | 1.0 | 2.0 | 8.0 | |
| 27 | 3 | C | C | C | 0.0 | 1.0 | 4.0 | 8.0 | |
| 28 | 3 | C | C | C | 0.0 | 1.0 | 8.0 | 8.0 | |
| 29 | 3 | C | C | C | 0.0 | -1.0 | 1.0 | 8.0 | |
| 30 | 3 | C | C | C | 0.0 | -1.0 | 2.0 | 8.0 | |
| 31 | 3 | C | C | C | 0.0 | -1.0 | 4.0 | 8.0 | |
| 32 | 3 | C | C | C | 0.0 | -1.0 | 8.0 | 8.0 | |
| 33 | 3 | C | H | H | 0.0 | 1.0 | 1.0 | 8.0 | |
| 34 | 3 | C | H | H | 0.0 | 1.0 | 2.0 | 8.0 | |
| 35 | 3 | C | H | H | 0.0 | 1.0 | 4.0 | 8.0 | |
| 36 | 3 | C | H | H | 0.0 | 1.0 | 8.0 | 8.0 | |
| 37 | 3 | C | H | H | 0.0 | -1.0 | 1.0 | 8.0 | |
| 38 | 3 | C | H | H | 0.0 | -1.0 | 2.0 | 8.0 | |
| 39 | 3 | C | H | H | 0.0 | -1.0 | 4.0 | 8.0 | |
| 40 | 3 | C | H | H | 0.0 | -1.0 | 8.0 | 8.0 | |
| 41 | 3 | C | C | H | 0.0 | 1.0 | 1.0 | 8.0 | |
| 42 | 3 | C | C | H | 0.0 | 1.0 | 2.0 | 8.0 | |
| 43 | 3 | C | C | H | 0.0 | 1.0 | 4.0 | 8.0 | |
| 44 | 3 | C | C | H | 0.0 | 1.0 | 8.0 | 8.0 | |
| 45 | 3 | C | C | H | 0.0 | -1.0 | 1.0 | 8.0 | |
| 46 | 3 | C | C | H | 0.0 | -1.0 | 2.0 | 8.0 | |
| 47 | 3 | C | C | H | 0.0 | -1.0 | 4.0 | 8.0 | |
| 48 | 3 | C | C | H | 0.0 | -1.0 | 8.0 | 8.0 | |
| 49 | 3 | H | C | C | 0.0 | 1.0 | 1.0 | 8.0 | |
| 50 | 3 | H | C | C | 0.0 | 1.0 | 2.0 | 8.0 | |
| 51 | 3 | H | C | C | 0.0 | 1.0 | 4.0 | 8.0 | |
| 52 | 3 | H | C | C | 0.0 | 1.0 | 8.0 | 8.0 | |
| 53 | 3 | H | C | C | 0.0 | -1.0 | 1.0 | 8.0 | |
| 54 | 3 | H | C | C | 0.0 | -1.0 | 2.0 | 8.0 | |
| 55 | 3 | H | H | C | 0.0 | 1.0 | 1.0 | 8.0 | |
| 56 | 3 | H | H | C | 0.0 | 1.0 | 2.0 | 8.0 | |
| 57 | 3 | H | H | C | 0.0 | 1.0 | 4.0 | 8.0 | |
| 58 | 3 | H | H | C | 0.0 | 1.0 | 8.0 | 8.0 | |
| 59 | 3 | H | H | C | 0.0 | -1.0 | 1.0 | 8.0 | |
| 60 | 3 | H | H | C | 0.0 | -1.0 | 2.0 | 8.0 | |

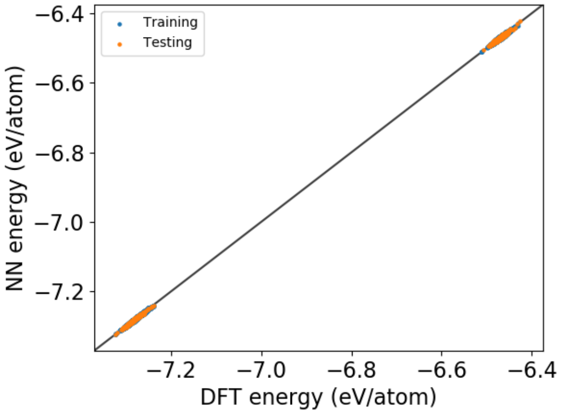


(a) 2G-HDNNP

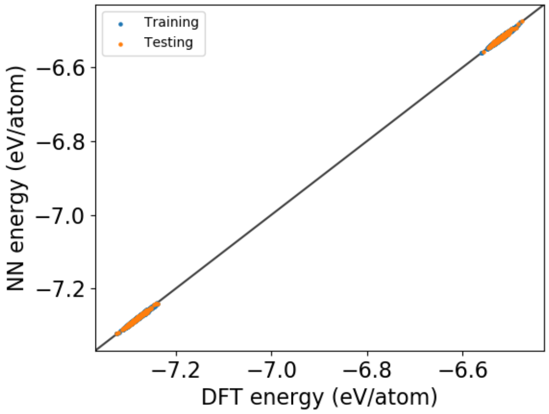


(b) 4G-HDNNP

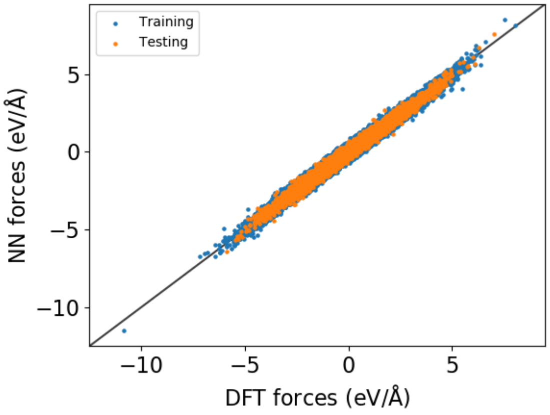


(c) 2G-HDNNP

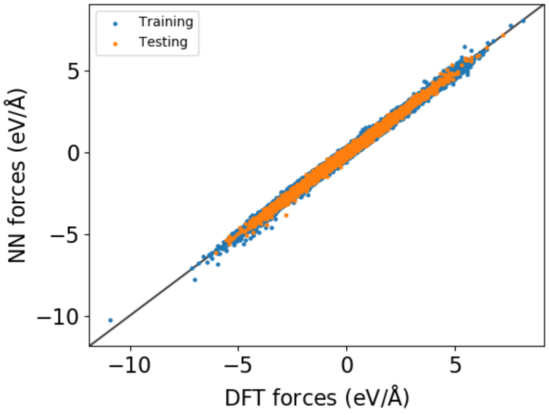


(d) 4G-HDNNP

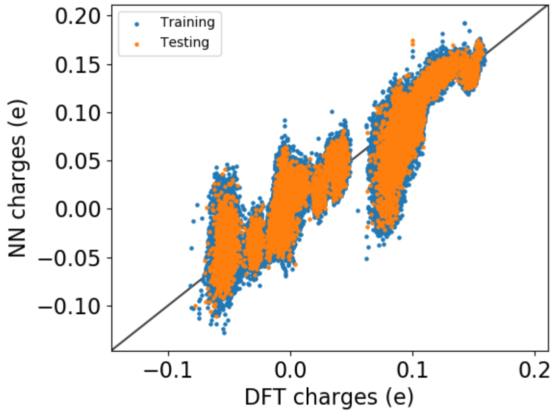


(e) 3G-HDNNP(scaled)

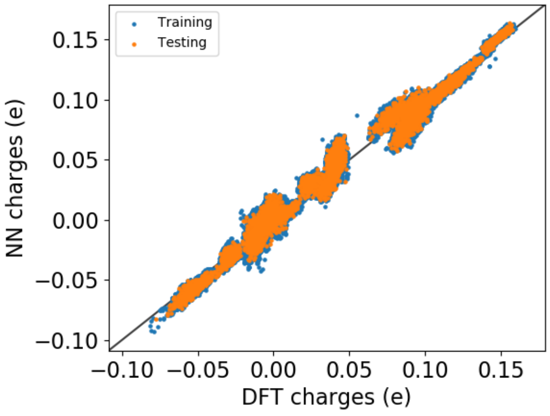


(f) 4G-HDNNP

Figure 1: Correlation plots for $C_{10}H_2/C_{10}H_3^+$

## 2.2 $Ag_3^{+/-}$ clusters

Table 3: Root mean square errors (RMSE) of charges (me), energies (meV/atom) and forces (meV/Å) for the three different HDNNP generations for the $Ag_3^{+/-}$ data set with 9930 and 1083 structures for training and testing points respectively.

| | | charges | energy | forces |
|---|---|---|---|---|
| 2G | train | — | 355.0 | 1812 |
| | test | — | 352.0 | 1803 |
| 3G (unscaled) | train | 75.50 | 345.0 | 1909 |
| | test | 77.55 | 340.0 | 1963 |
| 3G (scaled) | train | 26.24 | 321.1 | 1912 |
| | test | 26.48 | 320.2 | 1913 |
| 4G | train | 10.61 | 1.293 | 32.12 |
| | test | 9.976 | 1.323 | 31.69 |

Table 4: Symmetry functions for $Ag^{+/-}$ clusters

| no. | type | atom i | atom j | atom k | $\eta$(1/Bohr$^2$) | $\lambda$ | $\zeta$ | $R_c$(Bohr) | $R_s$(Bohr) |
|---|---|---|---|---|---|---|---|---|---|
| 1 | 2 | Ag | Ag | | 0.0 | | | 10.0 | 0.0 |
| 2 | 2 | Ag | Ag | | 0.007 | | | 10.0 | 0.0 |
| 3 | 2 | Ag | Ag | | 0.014 | | | 10.0 | 0.0 |
| 4 | 2 | Ag | Ag | | 0.025 | | | 10.0 | 0.0 |
| 5 | 2 | Ag | Ag | | 0.04 | | | 10.0 | 0.0 |
| 6 | 2 | Ag | Ag | | 0.062 | | | 10.0 | 0.0 |
| 7 | 3 | Ag | Ag | Ag | 0.0 | 1.0 | 1.0 | 10.0 | |
| 8 | 3 | Ag | Ag | Ag | 0.0 | 1.0 | 2.0 | 10.0 | |
| 9 | 3 | Ag | Ag | Ag | 0.0 | 1.0 | 4.0 | 10.0 | |
| 10 | 3 | Ag | Ag | Ag | 0.0 | 1.0 | 8.0 | 10.0 | |
| 11 | 3 | Ag | Ag | Ag | 0.0 | -1.0 | 1.0 | 10.0 | |
| 12 | 3 | Ag | Ag | Ag | 0.0 | -1.0 | 2.0 | 10.0 | |

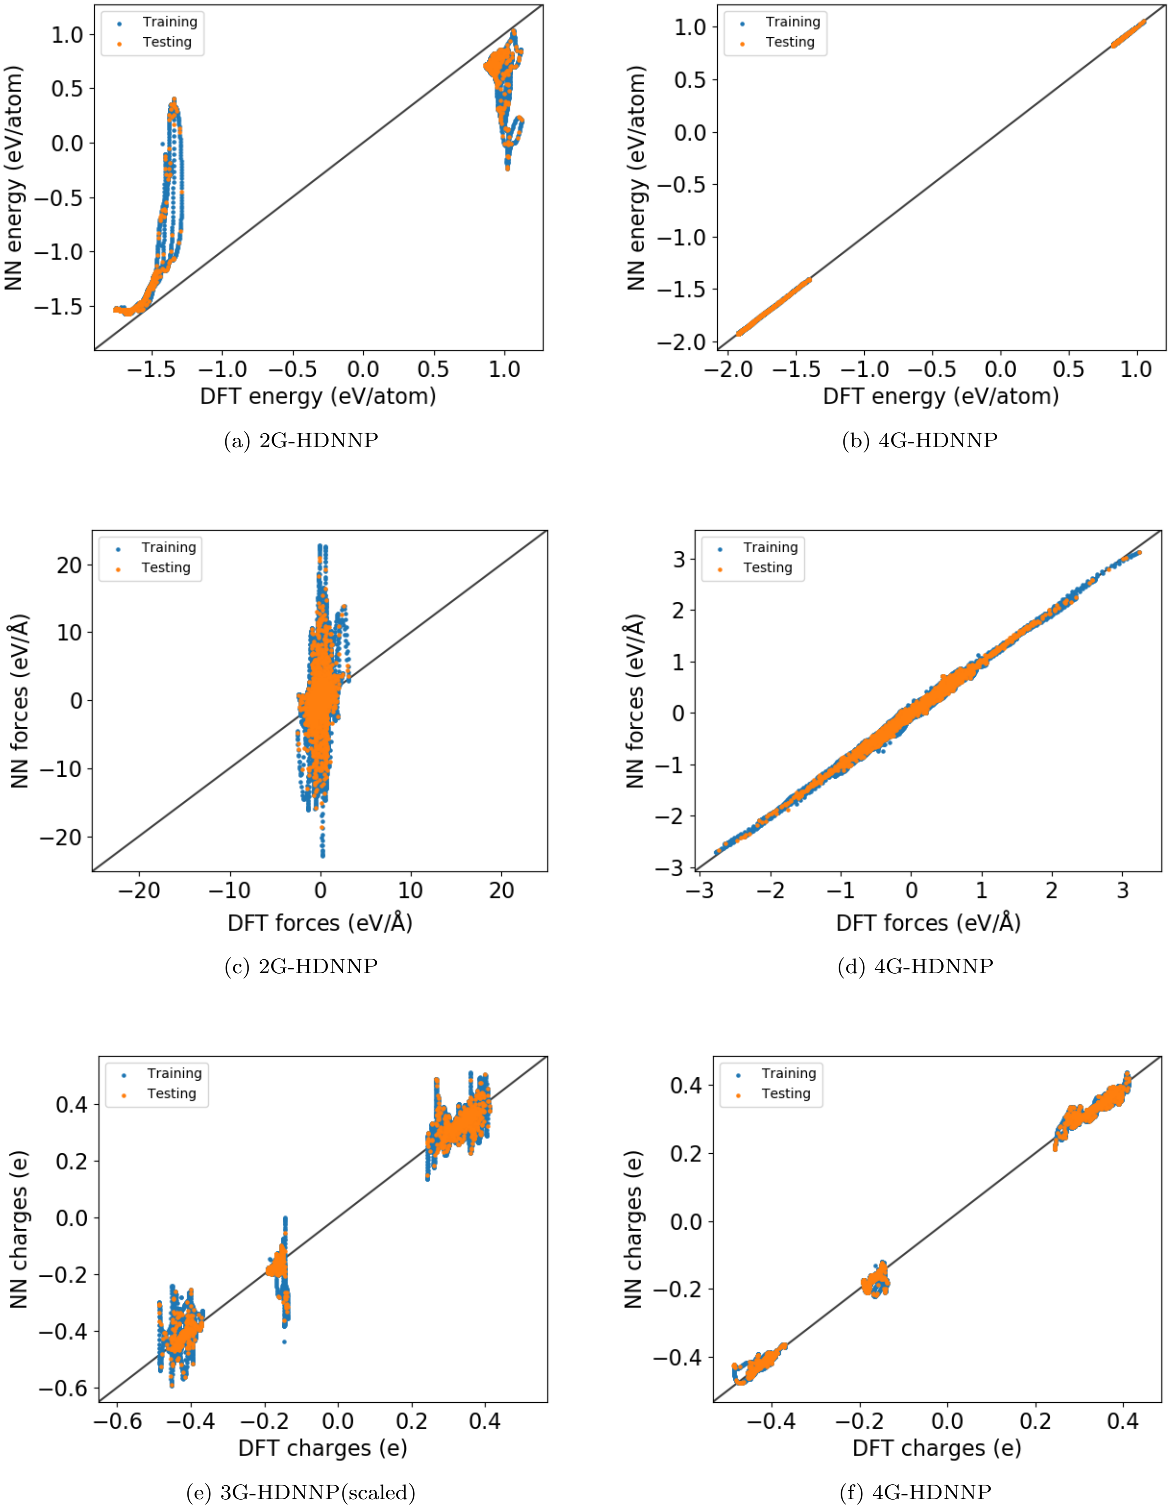


(a) 2G-HDNNP

(b) 4G-HDNNP

(c) 2G-HDNNP

(d) 4G-HDNNP

(e) 3G-HDNNP(scaled)

(f) 4G-HDNNP

Figure 2: Correlation plots for $Ag_3^{+/-}$

## 2.3 $Na_{8/9}Cl_8^+$ clusters

Table 5: Root mean square errors (RMSE) of charges (me), energies (meV/atom) and forces (meV/Å) for the three different HDNNP generations for the $Na_{8/9}Cl_8^+$ data set with 4493 and 507 structures for training and testing points respectively.

| | | charges | energy | forces |
|---|---|---|---|---|
| 2G | train | — | 1.690 | 57.54 |
| | test | — | 1.692 | 57.39 |
| 3G (unscaled) | train | 28.28 | 1.426 | 57.69 |
| | test | 28.52 | 1.470 | 59.49 |
| 3G (scaled) | train | 20.75 | 2.058 | 73.47 |
| | test | 20.80 | 2.042 | 76.67 |
| 4G | train | 15.87 | 0.474 | 32.45 |
| | test | 15.83 | 0.481 | 32.78 |

Table 6: Symmetry functions for $Na_{8/9}Cl_8^+$ clusters

| no. | type | atom i | atom j | atom k | $\eta$(1/Bohr$^2$) | $\lambda$ | $\zeta$ | $R_c$(Bohr) | $R_s$(Bohr) |
|---|---|---|---|---|---|---|---|---|---|
| 1 | 2 | Na | Na | | 0.0 | | | 10.0 | 0.0 |
| 2 | 2 | Na | Na | | 0.001 | | | 10.0 | 0.0 |
| 3 | 2 | Na | Na | | 0.002 | | | 10.0 | 0.0 |
| 4 | 2 | Na | Na | | 0.003 | | | 10.0 | 0.0 |
| 5 | 2 | Na | Na | | 0.004 | | | 10.0 | 0.0 |
| 6 | 2 | Na | Na | | 0.005 | | | 10.0 | 0.0 |
| 7 | 2 | Na | Cl | | 0.0 | | | 10.0 | 0.0 |
| 8 | 2 | Na | Cl | | 0.003 | | | 10.0 | 0.0 |
| 9 | 2 | Na | Cl | | 0.005 | | | 10.0 | 0.0 |
| 10 | 2 | Na | Cl | | 0.007 | | | 10.0 | 0.0 |
| 11 | 2 | Na | Cl | | 0.01 | | | 10.0 | 0.0 |
| 12 | 2 | Na | Cl | | 0.013 | | | 10.0 | 0.0 |
| 13 | 2 | Cl | Na | | 0.0 | | | 10.0 | 0.0 |
| 14 | 2 | Cl | Na | | 0.003 | | | 10.0 | 0.0 |
| 15 | 2 | Cl | Na | | 0.005 | | | 10.0 | 0.0 |
| 16 | 2 | Cl | Na | | 0.007 | | | 10.0 | 0.0 |
| 17 | 2 | Cl | Na | | 0.01 | | | 10.0 | 0.0 |
| 18 | 2 | Cl | Na | | 0.013 | | | 10.0 | 0.0 |
| 19 | 2 | Cl | Cl | | 0.0 | | | 10.0 | 0.0 |
| 20 | 2 | Cl | Cl | | 0.001 | | | 10.0 | 0.0 |
| 21 | 2 | Cl | Cl | | 0.002 | | | 10.0 | 0.0 |
| 22 | 2 | Cl | Cl | | 0.003 | | | 10.0 | 0.0 |
| 23 | 2 | Cl | Cl | | 0.004 | | | 10.0 | 0.0 |
| 24 | 2 | Cl | Cl | | 0.005 | | | 10.0 | 0.0 |

| no. | type | atom i | atom j | atom k | $\eta$(1/Bohr$^2$) | $\lambda$ | $\zeta$ | R$_c$(Bohr) | R$_s$(Bohr) |
|---|---|---|---|---|---|---|---|---|---|
| 25 | 3 | Na | Na | Cl | 0.0 | 1.0 | 1.0 | 10.0 | |
| 26 | 3 | Na | Na | Cl | 0.0 | 1.0 | 2.0 | 10.0 | |
| 27 | 3 | Na | Na | Cl | 0.0 | 1.0 | 4.0 | 10.0 | |
| 28 | 3 | Na | Na | Cl | 0.0 | 1.0 | 8.0 | 10.0 | |
| 29 | 3 | Na | Na | Cl | 0.0 | -1.0 | 1.0 | 10.0 | |
| 30 | 3 | Na | Na | Cl | 0.0 | -1.0 | 2.0 | 10.0 | |
| 31 | 3 | Na | Cl | Cl | 0.0 | 1.0 | 1.0 | 10.0 | |
| 32 | 3 | Na | Cl | Cl | 0.0 | 1.0 | 2.0 | 10.0 | |
| 33 | 3 | Na | Cl | Cl | 0.0 | -1.0 | 1.0 | 10.0 | |
| 34 | 3 | Na | Cl | Cl | 0.0 | -1.0 | 2.0 | 10.0 | |
| 35 | 3 | Na | Cl | Cl | 0.0 | -1.0 | 4.0 | 10.0 | |
| 36 | 3 | Cl | Cl | Na | 0.0 | 1.0 | 1.0 | 10.0 | |
| 37 | 3 | Cl | Cl | Na | 0.0 | 1.0 | 2.0 | 10.0 | |
| 38 | 3 | Cl | Cl | Na | 0.0 | 1.0 | 4.0 | 10.0 | |
| 39 | 3 | Cl | Cl | Na | 0.0 | 1.0 | 8.0 | 10.0 | |
| 40 | 3 | Cl | Cl | Na | 0.0 | -1.0 | 1.0 | 10.0 | |
| 41 | 3 | Cl | Na | Na | 0.0 | 1.0 | 1.0 | 10.0 | |
| 42 | 3 | Cl | Na | Na | 0.0 | 1.0 | 2.0 | 10.0 | |
| 43 | 3 | Cl | Na | Na | 0.0 | 1.0 | 4.0 | 10.0 | |
| 44 | 3 | Cl | Na | Na | 0.0 | -1.0 | 1.0 | 10.0 | |
| 45 | 3 | Cl | Na | Na | 0.0 | -1.0 | 2.0 | 10.0 | |

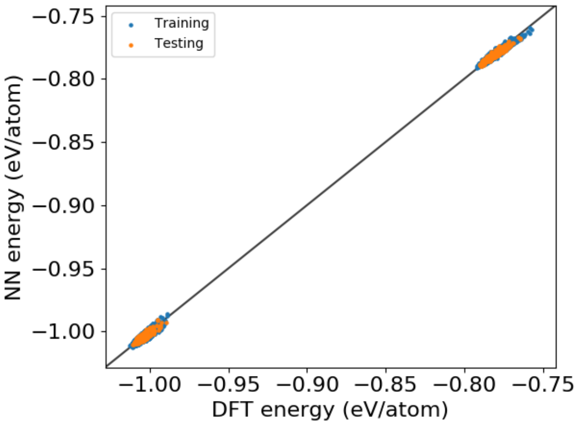


(a) 2G-HDNNP

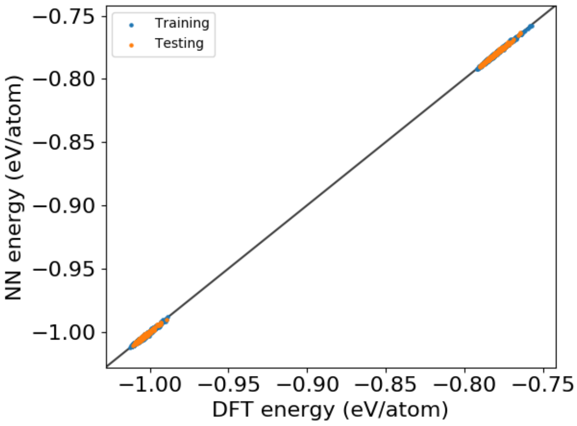


(b) 4G-HDNNP

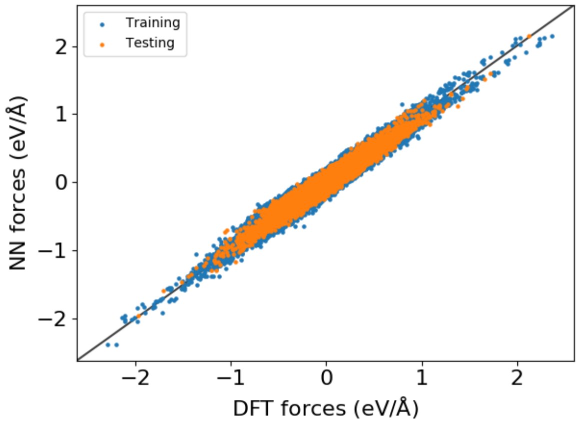


(c) 2G-HDNNP

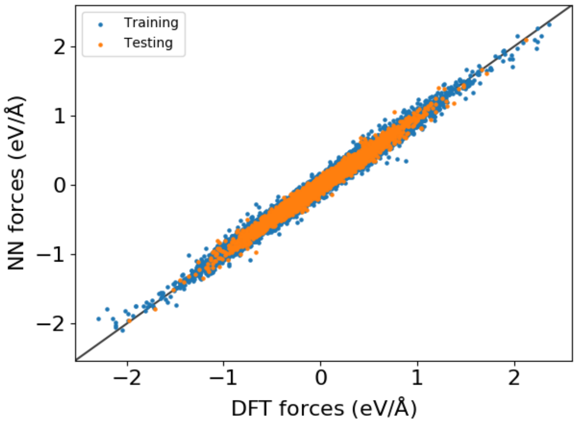


(d) 4G-HDNNP

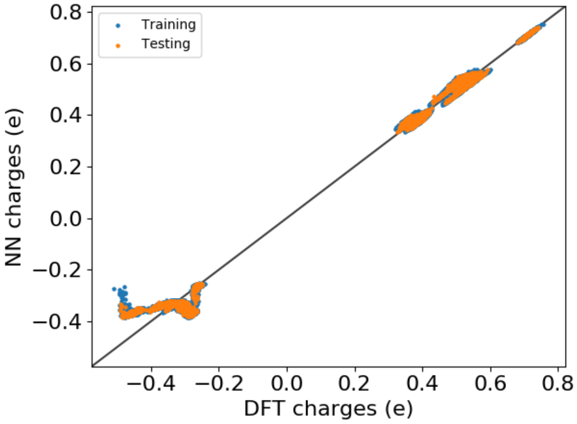


(e) 3G-HDNNP (unscaled)

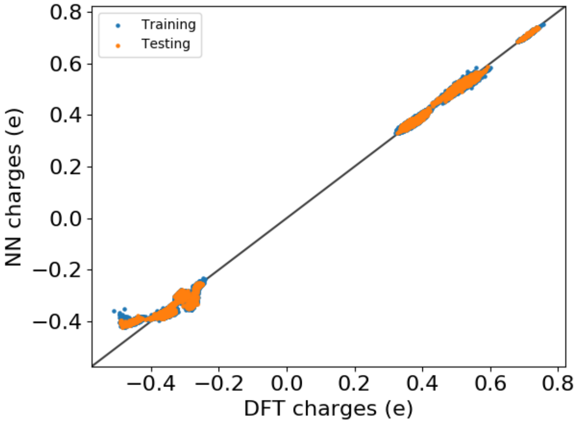


(f) 4G-HDNNP

Figure 3: Correlation plots for $Na_{8/9}Cl_8^+$

## 2.4 $Au_2$–MgO

Table 7: Root mean square errors (RMSE) of charges (me), energies (meV/atom) and forces (meV/Å) for the $Au_2$MgO data set with 4468 and 532 structures for training and testing points respectively.

| | | charges | energy | forces |
|---|---|---|---|---|
| 2G | train | — | 2.299 | 155.4 |
| | test | — | 2.287 | 153.1 |
| 4G | train | 5.663 | 0.209 | 81.05 |
| | test | 5.698 | 0.219 | 66.00 |

Table 8: Symmetry functions for $NaCl^+$ clusters

| no. | type | atom $i$ | atom $j$ | atom $k$ | $\eta$(1/Bohr$^2$) | $\lambda$ | $\zeta$ | $R_c$(Bohr) | $R_s$(Bohr) |
|---|---|---|---|---|---|---|---|---|---|
| 1 | 2 | Mg | Mg | | 0.0 | | | 8.0 | 0.0 |
| 2 | 2 | Mg | Mg | | 0.001 | | | 8.0 | 0.0 |
| 3 | 2 | Mg | Mg | | 0.002 | | | 8.0 | 0.0 |
| 4 | 2 | Mg | Mg | | 0.003 | | | 8.0 | 0.0 |
| 5 | 2 | Mg | Mg | | 0.004 | | | 8.0 | 0.0 |
| 6 | 2 | Mg | Mg | | 0.005 | | | 8.0 | 0.0 |
| 7 | 2 | O | Mg | | 0.0 | | | 8.0 | 0.0 |
| 8 | 2 | O | Mg | | 0.004 | | | 8.0 | 0.0 |
| 9 | 2 | O | Mg | | 0.007 | | | 8.0 | 0.0 |
| 10 | 2 | O | Mg | | 0.01 | | | 8.0 | 0.0 |
| 11 | 2 | O | Mg | | 0.014 | | | 8.0 | 0.0 |
| 12 | 2 | O | Mg | | 0.018 | | | 8.0 | 0.0 |
| 13 | 2 | Mg | O | | 0.0 | | | 8.0 | 0.0 |
| 14 | 2 | Mg | O | | 0.004 | | | 8.0 | 0.0 |
| 15 | 2 | Mg | O | | 0.007 | | | 8.0 | 0.0 |
| 16 | 2 | Mg | O | | 0.01 | | | 8.0 | 0.0 |
| 17 | 2 | Mg | O | | 0.014 | | | 8.0 | 0.0 |
| 18 | 2 | Mg | O | | 0.018 | | | 8.0 | 0.0 |
| 19 | 2 | O | O | | 0.0 | | | 8.0 | 0.0 |
| 20 | 2 | O | O | | 0.001 | | | 8.0 | 0.0 |
| 21 | 2 | O | O | | 0.002 | | | 8.0 | 0.0 |
| 22 | 2 | O | O | | 0.003 | | | 8.0 | 0.0 |
| 23 | 2 | O | O | | 0.004 | | | 8.0 | 0.0 |
| 24 | 2 | O | O | | 0.005 | | | 8.0 | 0.0 |
| 25 | 2 | Mg | Au | | 0.0 | | | 8.0 | 0.0 |
| 26 | 2 | Mg | Au | | 0.001 | | | 8.0 | 0.0 |
| 27 | 2 | Mg | Au | | 0.002 | | | 8.0 | 0.0 |
| 28 | 2 | Mg | Au | | 0.003 | | | 8.0 | 0.0 |

| no. | type | atom $i$ | atom $j$ | atom $k$ | $\eta(1/\text{Bohr}^2)$ | $\lambda$ | $\zeta$ | $R_\text{c}$(Bohr) | $R_\text{s}$(Bohr) |
|---|---|---|---|---|---|---|---|---|---|
| 29 | 2 | Mg | Au | | 0.004 | | | 8.0 | 0.0 |
| 30 | 2 | Mg | Au | | 0.005 | | | 8.0 | 0.0 |
| 31 | 2 | Au | Mg | | 0.0 | | | 8.0 | 0.0 |
| 32 | 2 | Au | Mg | | 0.001 | | | 8.0 | 0.0 |
| 33 | 2 | Au | Mg | | 0.002 | | | 8.0 | 0.0 |
| 34 | 2 | Au | Mg | | 0.003 | | | 8.0 | 0.0 |
| 35 | 2 | Au | Mg | | 0.004 | | | 8.0 | 0.0 |
| 36 | 2 | Au | Mg | | 0.005 | | | 8.0 | 0.0 |
| 37 | 2 | Au | O | | 0.0 | | | 8.0 | 0.0 |
| 38 | 2 | Au | O | | 0.004 | | | 8.0 | 0.0 |
| 39 | 2 | Au | O | | 0.008 | | | 8.0 | 0.0 |
| 40 | 2 | Au | O | | 0.013 | | | 8.0 | 0.0 |
| 41 | 2 | Au | O | | 0.018 | | | 8.0 | 0.0 |
| 42 | 2 | Au | O | | 0.024 | | | 8.0 | 0.0 |
| 43 | 2 | O | Au | | 0.0 | | | 8.0 | 0.0 |
| 44 | 2 | O | Au | | 0.004 | | | 8.0 | 0.0 |
| 45 | 2 | O | Au | | 0.008 | | | 8.0 | 0.0 |
| 46 | 2 | O | Au | | 0.013 | | | 8.0 | 0.0 |
| 47 | 2 | O | Au | | 0.018 | | | 8.0 | 0.0 |
| 48 | 2 | O | Au | | 0.024 | | | 8.0 | 0.0 |
| 49 | 2 | Au | Au | | 0.0 | | | 8.0 | 0.0 |
| 50 | 2 | Au | Au | | 0.004 | | | 8.0 | 0.0 |
| 51 | 2 | Au | Au | | 0.008 | | | 8.0 | 0.0 |
| 52 | 2 | Au | Au | | 0.012 | | | 8.0 | 0.0 |
| 53 | 2 | Au | Au | | 0.017 | | | 8.0 | 0.0 |
| 54 | 2 | Au | Au | | 0.022 | | | 8.0 | 0.0 |
| 55 | 2 | O | Al | | 0.0 | | | 8.0 | 0.0 |
| 56 | 2 | O | Al | | 0.003 | | | 8.0 | 0.0 |
| 57 | 2 | O | Al | | 0.005 | | | 8.0 | 0.0 |
| 58 | 2 | O | Al | | 0.008 | | | 8.0 | 0.0 |
| 59 | 2 | O | Al | | 0.011 | | | 8.0 | 0.0 |
| 60 | 2 | O | Al | | 0.014 | | | 8.0 | 0.0 |
| 61 | 2 | Al | O | | 0.0 | | | 8.0 | 0.0 |
| 62 | 2 | Al | O | | 0.003 | | | 8.0 | 0.0 |
| 63 | 2 | Al | O | | 0.005 | | | 8.0 | 0.0 |
| 64 | 2 | Al | O | | 0.008 | | | 8.0 | 0.0 |
| 65 | 2 | Al | O | | 0.011 | | | 8.0 | 0.0 |
| 66 | 2 | Al | O | | 0.014 | | | 8.0 | 0.0 |
| 67 | 2 | Al | Mg | | 0.0 | | | 8.0 | 0.0 |
| 68 | 2 | Al | Mg | | 0.001 | | | 8.0 | 0.0 |
| 69 | 2 | Al | Mg | | 0.002 | | | 8.0 | 0.0 |
| 70 | 2 | Al | Mg | | 0.003 | | | 8.0 | 0.0 |
| 71 | 2 | Al | Mg | | 0.004 | | | 8.0 | 0.0 |
| 72 | 2 | Al | Mg | | 0.005 | | | 8.0 | 0.0 |

| no. | type | atom $i$ | atom $j$ | atom $k$ | $\eta(1/\mathrm{Bohr}^2)$ | $\lambda$ | $\zeta$ | $R_\mathrm{c}$(Bohr) | $R_\mathrm{s}$(Bohr) |
|---|---|---|---|---|---|---|---|---|---|
| 73 | 2 | Mg | Al | | 0.0 | | | 8.0 | 0.0 |
| 74 | 2 | Mg | Al | | 0.001 | | | 8.0 | 0.0 |
| 75 | 2 | Mg | Al | | 0.002 | | | 8.0 | 0.0 |
| 76 | 2 | Mg | Al | | 0.003 | | | 8.0 | 0.0 |
| 77 | 2 | Mg | Al | | 0.004 | | | 8.0 | 0.0 |
| 78 | 2 | Mg | Al | | 0.005 | | | 8.0 | 0.0 |
| 79 | 3 | Mg | Mg | Mg | 0.0 | 1.0 | 1.0 | 8.0 | |
| 80 | 3 | Mg | Mg | Mg | 0.0 | 1.0 | 2.0 | 8.0 | |
| 81 | 3 | Mg | Mg | Mg | 0.0 | 1.0 | 4.0 | 8.0 | |
| 82 | 3 | Mg | Mg | Mg | 0.0 | -1.0 | 1.0 | 8.0 | |
| 83 | 3 | Mg | Mg | O | 0.0 | 1.0 | 1.0 | 8.0 | |
| 84 | 3 | Mg | Mg | O | 0.0 | 1.0 | 2.0 | 8.0 | |
| 85 | 3 | Mg | Mg | O | 0.0 | 1.0 | 4.0 | 8.0 | |
| 86 | 3 | Mg | Mg | O | 0.0 | 1.0 | 8.0 | 8.0 | |
| 87 | 3 | Mg | Mg | O | 0.0 | -1.0 | 1.0 | 8.0 | |
| 88 | 3 | Mg | Mg | O | 0.0 | -1.0 | 2.0 | 8.0 | |
| 89 | 3 | Mg | O | O | 0.0 | 1.0 | 1.0 | 8.0 | |
| 90 | 3 | Mg | O | O | 0.0 | 1.0 | 2.0 | 8.0 | |
| 91 | 3 | Mg | O | O | 0.0 | 1.0 | 4.0 | 8.0 | |
| 92 | 3 | Mg | O | O | 0.0 | -1.0 | 1.0 | 8.0 | |
| 93 | 3 | Mg | O | O | 0.0 | -1.0 | 2.0 | 8.0 | |
| 94 | 3 | Mg | O | O | 0.0 | -1.0 | 4.0 | 8.0 | |
| 95 | 3 | Mg | O | Al | 0.0 | 1.0 | 1.0 | 8.0 | |
| 96 | 3 | Mg | O | Al | 0.0 | 1.0 | 2.0 | 8.0 | |
| 97 | 3 | Mg | O | Al | 0.0 | 1.0 | 4.0 | 8.0 | |
| 98 | 3 | Mg | O | Al | 0.0 | 1.0 | 8.0 | 8.0 | |
| 99 | 3 | Mg | O | Al | 0.0 | -1.0 | 1.0 | 8.0 | |
| 100 | 3 | Mg | O | Au | 0.0 | 1.0 | 1.0 | 8.0 | |
| 101 | 3 | Mg | O | Au | 0.0 | 1.0 | 2.0 | 8.0 | |
| 102 | 3 | Mg | O | Au | 0.0 | 1.0 | 4.0 | 8.0 | |
| 103 | 3 | Mg | O | Au | 0.0 | 1.0 | 8.0 | 8.0 | |
| 104 | 3 | Mg | O | Au | 0.0 | -1.0 | 1.0 | 8.0 | |
| 105 | 3 | Mg | O | Au | 0.0 | -1.0 | 2.0 | 8.0 | |
| 106 | 3 | O | Mg | Mg | 0.0 | 1.0 | 1.0 | 8.0 | |
| 107 | 3 | O | Mg | Mg | 0.0 | 1.0 | 2.0 | 8.0 | |
| 108 | 3 | O | Mg | Mg | 0.0 | 1.0 | 4.0 | 8.0 | |
| 109 | 3 | O | Mg | Mg | 0.0 | -1.0 | 1.0 | 8.0 | |
| 110 | 3 | O | Mg | Mg | 0.0 | -1.0 | 2.0 | 8.0 | |
| 111 | 3 | O | Mg | Mg | 0.0 | -1.0 | 4.0 | 8.0 | |
| 112 | 3 | O | Mg | O | 0.0 | 1.0 | 1.0 | 8.0 | |
| 113 | 3 | O | Mg | O | 0.0 | 1.0 | 2.0 | 8.0 | |
| 114 | 3 | O | Mg | O | 0.0 | 1.0 | 4.0 | 8.0 | |
| 115 | 3 | O | Mg | O | 0.0 | 1.0 | 8.0 | 8.0 | |
| 116 | 3 | O | Mg | O | 0.0 | -1.0 | 1.0 | 8.0 | |

| no. | type | atom $i$ | atom $j$ | atom $k$ | $\eta$(1/Bohr$^2$) | $\lambda$ | $\zeta$ | $R_c$(Bohr) | $R_s$(Bohr) |
|---|---|---|---|---|---|---|---|---|---|
| 117 | 3 | O | Mg | O | 0.0 | -1.0 | 2.0 | 8.0 | |
| 118 | 3 | O | Mg | Al | 0.0 | 1.0 | 1.0 | 8.0 | |
| 119 | 3 | O | Mg | Al | 0.0 | 1.0 | 2.0 | 8.0 | |
| 120 | 3 | O | Mg | Al | 0.0 | 1.0 | 4.0 | 8.0 | |
| 121 | 3 | O | Mg | Al | 0.0 | -1.0 | 1.0 | 8.0 | |
| 122 | 3 | O | Mg | Al | 0.0 | -1.0 | 2.0 | 8.0 | |
| 123 | 3 | O | Mg | Al | 0.0 | -1.0 | 4.0 | 8.0 | |
| 124 | 3 | O | Mg | Au | 0.0 | 1.0 | 1.0 | 8.0 | |
| 125 | 3 | O | Mg | Au | 0.0 | 1.0 | 2.0 | 8.0 | |
| 126 | 3 | O | Mg | Au | 0.0 | -1.0 | 1.0 | 8.0 | |
| 127 | 3 | O | Mg | Au | 0.0 | -1.0 | 2.0 | 8.0 | |
| 128 | 3 | O | O | O | 0.0 | 1.0 | 1.0 | 8.0 | |
| 129 | 3 | O | O | O | 0.0 | 1.0 | 2.0 | 8.0 | |
| 130 | 3 | O | O | O | 0.0 | -1.0 | 1.0 | 8.0 | |
| 131 | 3 | O | O | Al | 0.0 | 1.0 | 1.0 | 8.0 | |
| 132 | 3 | O | O | Al | 0.0 | 1.0 | 2.0 | 8.0 | |
| 133 | 3 | O | O | Al | 0.0 | -1.0 | 1.0 | 8.0 | |
| 134 | 3 | O | O | Al | 0.0 | -1.0 | 2.0 | 8.0 | |
| 135 | 3 | Al | Mg | Mg | 0.0 | 1.0 | 1.0 | 8.0 | |
| 136 | 3 | Al | Mg | O | 0.0 | 1.0 | 1.0 | 8.0 | |
| 137 | 3 | Al | Mg | O | 0.0 | 1.0 | 2.0 | 8.0 | |
| 138 | 3 | Al | Mg | O | 0.0 | -1.0 | 1.0 | 8.0 | |
| 139 | 3 | Al | O | O | 0.0 | 1.0 | 1.0 | 8.0 | |
| 140 | 3 | Al | O | O | 0.0 | 1.0 | 2.0 | 8.0 | |
| 141 | 3 | Al | O | O | 0.0 | -1.0 | 1.0 | 8.0 | |
| 142 | 3 | Al | O | O | 0.0 | -1.0 | 2.0 | 8.0 | |
| 143 | 3 | Au | Mg | Mg | 0.0 | 1.0 | 1.0 | 8.0 | |
| 144 | 3 | Au | Mg | Mg | 0.0 | 1.0 | 2.0 | 8.0 | |
| 145 | 3 | Au | Mg | O | 0.0 | 1.0 | 1.0 | 8.0 | |
| 146 | 3 | Au | Mg | O | 0.0 | 1.0 | 2.0 | 8.0 | |
| 147 | 3 | Au | Mg | O | 0.0 | -1.0 | 1.0 | 8.0 | |
| 148 | 3 | Au | Mg | O | 0.0 | -1.0 | 2.0 | 8.0 | |
| 149 | 3 | Au | O | O | 0.0 | 1.0 | 1.0 | 8.0 | |
| 150 | 3 | Au | O | Au | 0.0 | 1.0 | -1.0 | 8.0 | |
| 151 | 3 | Au | O | Au | 0.0 | 1.0 | -2.0 | 8.0 | |

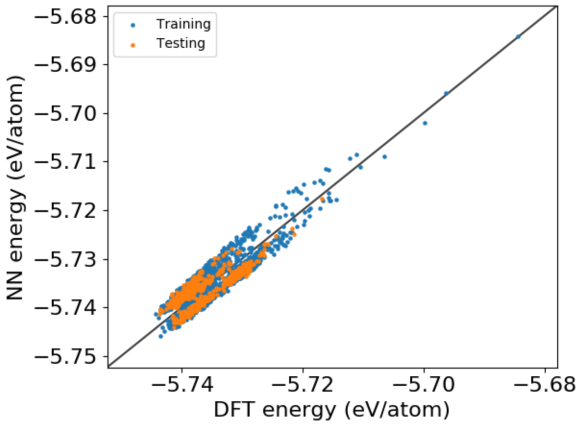


(a) 2G-HDNNP

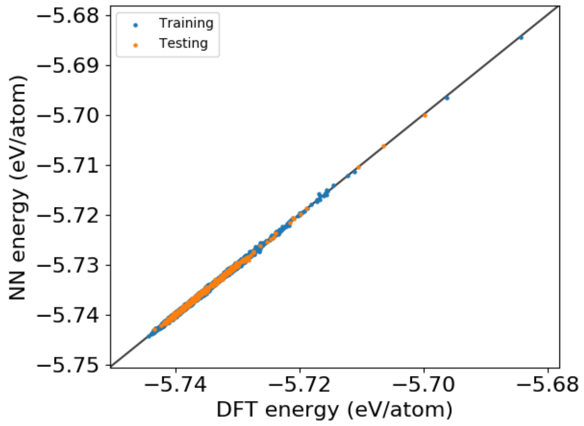


(b) 4G-HDNNP

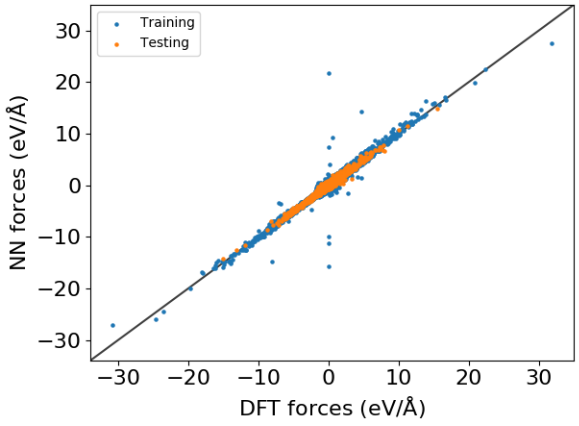


(c) 2G-HDNNP

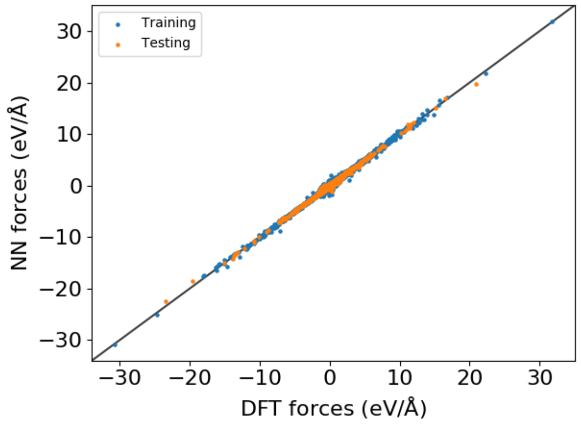


(d) 4G-HDNNP

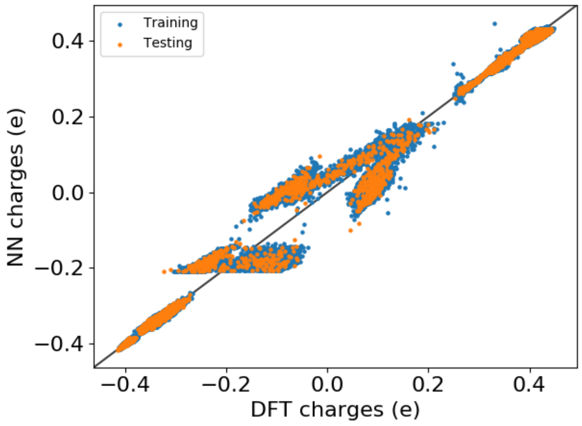


(e) 3G-HDNNP (scaled)

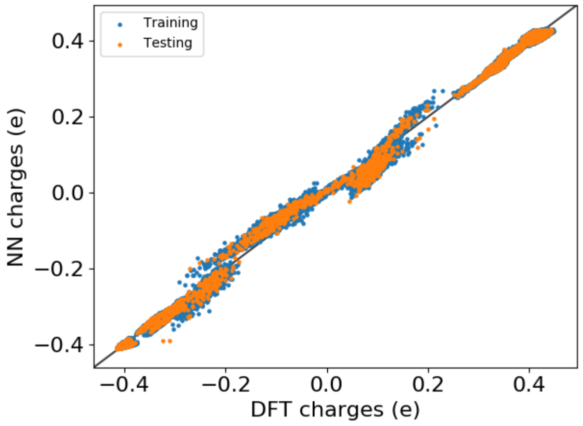


(f) 4G-HDNNP

Figure 4: Correlation plots for $Au_2MgO$

# 3 DFT-optimized geometries

## 3.1 $C_{10}H_2/C_{10}H_3^+$

Table 9: DFT-optimized structure of $C_{10}H_2$ in XYZ format (distance unit in Å)

12 atoms

| | | | |
|---|---|---|---|
| C | 0.621 587 11 | 0.000 000 00 | 0.000 000 00 |
| C | −0.621 587 10 | 0.000 000 00 | 0.000 000 00 |
| C | 1.952 478 40 | 0.000 000 00 | 0.000 000 00 |
| C | −1.952 478 47 | 0.000 000 00 | 0.000 000 00 |
| C | 3.192 145 71 | 0.000 000 00 | 0.000 000 00 |
| C | −3.192 145 71 | 0.000 000 00 | 0.000 000 00 |
| C | 4.535 930 62 | 0.000 000 00 | 0.000 000 00 |
| C | −4.535 930 61 | 0.000 000 00 | 0.000 000 00 |
| C | 5.761 179 51 | 0.000 000 00 | 0.000 000 00 |
| C | −5.761 179 49 | 0.000 000 00 | 0.000 000 00 |
| H | 6.831 800 63 | 0.000 000 00 | 0.000 000 00 |
| H | −6.831 800 59 | 0.000 000 00 | 0.000 000 00 |

Table 10: DFT-optimized structure of $C_{10}H_3^+$ in XYZ format (distance unit in Å)

13 atoms

| | | | |
|---|---|---|---|
| C | 0.629 569 25 | 0.000 007 77 | 0.000 008 66 |
| C | −0.630 171 87 | 0.000 006 61 | 0.000 007 49 |
| C | 1.927 800 72 | 0.000 005 14 | 0.000 005 65 |
| C | −1.939 451 25 | 0.000 003 66 | 0.000 004 44 |
| C | 3.196 698 75 | −0.000 004 40 | −0.000 004 75 |
| C | −3.188 248 16 | 0.000 001 20 | 0.000 001 93 |
| C | 4.485 686 49 | −0.000 026 21 | −0.000 028 65 |
| C | −4.518 203 60 | −0.000 000 93 | −0.000 000 22 |
| C | 5.792 415 11 | −0.000 049 55 | −0.000 059 76 |
| C | −5.745 974 58 | −0.000 002 54 | −0.000 001 78 |
| H | 6.356 582 33 | 0.664 760 64 | −0.662 349 90 |
| H | −6.821 318 48 | −0.000 003 46 | −0.000 002 64 |
| H | 6.356 596 39 | −0.664 669 86 | 0.662 408 63 |

Table 11: DFT-optimized structure of $Ag_3^+$ in XYZ format (distance unit in Å)

3 atoms

| | | | |
|---|---|---|---|
| Ag | 0.000 000 00 | 0.000 644 41 | 1.556 755 15 |
| Ag | 0.000 000 00 | 1.347 626 41 | −0.779 404 15 |
| Ag | 0.000 000 00 | −1.348 270 81 | −0.777 351 99 |

Table 12: DFT-optimized structure of $Ag_3^-$ in XYZ format (distance unit in Å)

3 atoms

| | | | |
|---|---|---|---|
| Ag | 0.000 000 00 | −1.326 870 06 | 2.317 857 81 |
| Ag | 0.000 000 00 | 1.340 265 98 | −2.309 774 04 |
| Ag | 0.000 000 00 | −0.013 395 92 | −0.008 084 77 |

Table 13: DFT-optimized structure of $Na_9Cl_8^+$ in XYZ format (distance unit in Å)

17 atoms

| | | | |
|---|---|---|---|
| Na | −4.672 483 91 | 1.744 323 61 | 0.066 917 32 |
| Cl | −4.674 131 38 | −0.763 117 13 | −0.005 394 92 |
| Cl | −2.156 850 54 | 2.353 451 40 | 0.126 851 59 |
| Na | −2.120 583 99 | −0.453 759 70 | 0.037 785 66 |
| Na | 0.430 089 05 | 2.067 507 92 | 0.061 237 48 |
| Cl | 0.514 739 28 | −0.620 487 80 | 0.003 580 16 |
| Cl | 3.054 771 88 | 2.435 379 02 | 0.005 454 56 |
| Na | 3.081 187 44 | −0.275 178 18 | −0.020 881 71 |
| Na | 5.635 084 96 | 2.195 983 30 | −0.008 956 06 |
| Cl | 5.728 609 48 | −0.495 161 62 | −0.005 581 27 |
| Cl | 8.304 179 09 | 2.518 938 87 | 0.008 721 19 |
| Na | 15.163 008 08 | 4.522 166 97 | −0.019 004 50 |
| Na | 10.847 244 50 | 2.274 841 80 | −0.037 879 82 |
| Cl | 10.992 739 88 | −0.383 182 02 | −0.002 413 13 |
| Cl | 13.644 077 08 | 2.525 223 09 | 0.039 396 59 |
| Na | 13.502 039 57 | −0.152 682 89 | 0.114 915 06 |
| Na | 8.284 823 01 | −0.197 007 56 | 0.036 113 70 |

# References


[1] A. K. Rappe and W. A. Goddard, III, J. Phys. Chem. **95**, 3358 (1991).

[2] P. P. Poier, L. Lagardère, J.-P. Piquemal, and F. Jensen, J. Chem. Theory Comput. **15**, 6213 (2019).

[3] P. P. Ewald, Annalen der physik **369**, 253 (1921).

[4] T. R. Gingrich and M. Wilson, Chem. Phys. Lett. **500**, 178 (2010).

[5] P. T. Kiss, M. Sega, and A. Baranyai, J. Chem. Theory Comput. **10**, 5513 (2014).

[6] H. Lee and W. Cai, Lecture Notes, Stanford University (2009).
